# Supplementary material for: Effect Summaries for Thread-Modular Analysis
Source: arXiv:1705.03701 source file (2017-05-10)
Supplement: Supplementary file 1 [file proofs.tex]

%!TEX root = ../../main.tex

\section{Missing Proofs (old)}

This section contains missing proofs and auxiliary statements.
For clarity, we extend the program steps, $\!\stepprog\!$, from \cref{sec:programming-model} by a subscript $i$, \ie, $\!\stepprog[i]\!$, in order to denote that thread $i$ is performing the step.

%%%%%%%%%%%%%%%%%%%%%%%%%%%%%%%%%%%%%%%%%%%%%%%%%%%%%%%%%%%%%%%%%%%%%%%%%%%%%%
%%%%%%%%%%%%%%%%%%%%%%%%%%%%%%%%%%%%%%%%%%%%%%%%%%%%%%%%%%%%%%%%%%%%%%%%%%%%%%
%%%%%%%%%%%%%%%%%%%%%%%%%%%%%%%%%%%%%%%%%%%%%%%%%%%%%%%%%%%%%%%%%%%%%%%%%%%%%%

\subsection{Auxiliaries}

\begin{lemma}
	\label{auxthm:stateless-does-not-care-for-duplicated-threads}
	Let $\EBNFprogramQ$ be a program with $\stateless[]{\EBNFprogramQ}$.
	Let $\EBNFthread\in\EBNFprogramQ$ be one of its threads.
	Then, $\ReachEff[]{\EBNFthread\inpar\EBNFprogramQ^*}\subseteq\ReachEff[]{\EBNFprogramQ^*}$.
\end{lemma}

\begin{lemma}
	\label{auxthm:stateless-effects-give-repeated-executions}
	Let $\EBNFprogramQ$ be a program with $\stateless[]{\EBNFprogramQ}$.
	For every $\pair{s}{s'}\in\ReachEff[]{\EBNFprogramQ^*}$ we have $\state{s}{\cfinit{\EBNFprogramQ^*}}\stepprogany\state{s'}{\cfinit{\EBNFprogramQ^*}}$.
\end{lemma}

\begin{proof}[\Cref{auxthm:stateless-does-not-care-for-duplicated-threads}]
	Let $\EBNFprogramQ$ be a stateless program and let $\EBNFthread\in\EBNFprogramQ$ be one of its threads.
	Without loss of generality, let
	\begin{gather*}
		\cfinit{\EBNFthread\inpar\EBNFprogramQ^*}=\set{0\mapsto\conf{\EBNFthread}{\emp}}\uplus\cfinit{\EBNFprogramQ^*}
	\end{gather*}
	to avoid remapping thread identifiers of different programs.
	We proceed by induction.
	
	\begin{description}[labelwidth=6mm,leftmargin=8mm,itemindent=0mm]
		\item[IB:]
			The claim is trivially true.
			\\[-2mm]

		\item[IH:]
			For every $\init{\EBNFthread\inpar\EBNFprogramQ^*}\stepprogany\state{s}{\cf}$ we have
			\begin{compactitem}
			 	\item $\init{\EBNFprogramQ^*}\stepprogany\state{s}{\cfinit{\EBNFprogramQ^*}}$
			 	\item $\cf(0)\in\set{\conf{\EBNFthread}{\emp},\conf{\cmdskip}{\emp}}$
			 	\item $\cf(i)\in\set{\conf{\cmdskip}{\emp},\conf{\cmdskip;\EBNFthread_i^*}{\emp},\conf{\EBNFthread_i^*}{\emp},\conf{\EBNFthread_i;\EBNFthread_i^*}{\emp}}$ for every $i,\EBNFthread_i$ with $\cfinit{\EBNFprogramQ^*}(i)=\conf{\EBNFthread_i}{\emp}$
			 	\\[-2mm]
			\end{compactitem}

		\item[IS:]
			Consider now $\init{\EBNFthread\inpar\EBNFprogramQ^*}\stepprogany\state{s}{\cf}\stepprog[i]\state{s'}{\cf'}$ for some $i$.
			By the semantics we have $\cf(j)=\cf'(j)$ for all $j\neq i$.
			Hence, the second and third proof obligation boil down to showing that $\cf'(i)$ has the appropriate form.
			We do a case distinction on $i$.
			\\[-2mm]

			\textit{Case $i = 0$.}
			By induction we must have $\cf(0)\!=\!\conf{\EBNFthread}{\emp}$ with $\EBNFthread\not\equiv\cmdskip$ as for otherwise the last step would not be possible.
			The induction hypothesis also provides $\init{\EBNFprogramQ^*}\stepprogany\state{s}{\cfinit{\EBNFprogramQ^*}}$.
			That is, $s\in\Reach{\EBNFprogramQ^*}$.
			Due to $\stateless[]{\EBNFprogramQ^*}$ and $\EBNFthread\in\EBNFprogramQ$ we have $\cf'(0)=\conf{\cmdskip}{\emp}$.
			So $\cf'$ has the appropriate form.
			So $\state{s}{\conf{\EBNFthread}{\emp}}\stepprog\state{s'}{\conf{\cmdskip}{\emp}}$ by the semantics and thus:
			\begin{align*}
				\state{s}{\conf{\EBNFthread^*}{\emp}}
				\stepprog
				&\state{s}{\conf{\EBNFthread;\EBNFthread^*}{\emp}}
				\stepprog
				\state{s'}{\conf{\cmdskip;\EBNFthread^*}{\emp}}\\
				\stepprog
				&\state{s'}{\conf{\EBNFthread^*}{\emp}}
			\end{align*}
			By $\EBNFthread\in\EBNFprogramQ$ this yields $\init{\EBNFprogramQ^*}\stepprogany\state{s}{\cfinit{\EBNFprogramQ^*}}\stepprogany\state{s'}{\cfinit{\EBNFprogramQ^*}}$.
			This concludes the case.
			\\[-2mm]

			\textit{Case $i \neq 0$.}
			By the semantics we cannot have $\cf(i)=\conf{\cmdskip}{\emp}$.
			For the case $\cf(i)\in\set{\conf{\cmdskip;\EBNFthread_i^*}{\emp},\conf{\EBNFthread_i^*}{\emp}}$ we immediately get $s=s'$, thus $\init{\EBNFprogramQ^*}\stepprogany\state{s'}{\cfinit{\EBNFprogramQ^*}}$, and the desired form of $\cf'$.
			It remains to consider $\cf(i)=\conf{\EBNFthread_i;\EBNFthread_i^*}{\emp}$ with $\EBNFthread_i\not\equiv\cmdskip$.
			Due to the semantics and statelessness of $\EBNFprogramQ$ we have $\state{s}{\conf{\EBNFthread_i}{\emp}}\stepprog\state{s'}{\conf{\cmdskip}{\emp}}$.
			Hence, we know that $\cf'(i)=\conf{\cmdskip;\EBNFthread_i^*}{\emp}$ is of the proper form.
			And similarly to the previous case we get:
			\begin{align*}
				\state{s}{\conf{\EBNFthread_i^*}{\emp}}
				\stepprog
				&\state{s}{\conf{\EBNFthread_i;\EBNFthread_i^*}{\emp}}
				\stepprog
				\state{s'}{\conf{\cmdskip;\EBNFthread_i^*}{\emp}}\\
				\stepprog
				&\state{s'}{\conf{\EBNFthread_i^*}{\emp}}
			\end{align*}
			By $\EBNFthread_i\in\EBNFprogramQ$ this yields $\init{\EBNFprogramQ^*}\stepprogany\state{s}{\cfinit{\EBNFprogramQ^*}}\stepprogany\state{s'}{\cfinit{\EBNFprogramQ^*}}$.
			This concludes the claim.
	\end{description}
\end{proof}

\begin{proof}[\Cref{auxthm:stateless-effects-give-repeated-executions}]
	Let $\EBNFprogramQ$ be a program with $\stateless[]{\EBNFprogramQ}$.
	Let $\pair{s}{s'}\in\ReachEff[]{\EBNFprogramQ^*}$ be an effect with $s\neq s'$ as nothing needs to be shown otherwise.
	Consider now $\EBNFprogramQ'=\cmdskip\inpar\EBNFprogramQ$.
	Obviously, $\pair{s}{s'}\in\ReachEff[]{\EBNFprogramQ^*}$.
	So there is an execution of the form $\init{\cmdskip\inpar\EBNFprogramQ^*}\stepprogany\state{s}{\cf}\stepprog[i]\state{s'}{\cf'}$ for some $i$.
	By the induction from the Proof of \cref{auxthm:stateless-does-not-care-for-duplicated-threads} together with the semantics we must have $\cf(i)=\conf{\EBNFthread;\EBNFthread^*}{\emp}$ and $\cf'(i)=\conf{\cmdskip;\EBNFthread^*}{\emp}$ with $\EBNFthread\not\equiv\cmdskip$ such that $\cfinit{\EBNFprogramQ^*}(i)=\conf{\EBNFthread}{\emp}$.
	So the following is valid:
	\begin{align*}
		\state{s}{\conf{\EBNFthread^*}{\emp}}
		\stepprog
		&\state{s}{\conf{\EBNFthread;\EBNFthread^*}{\emp}}
		\stepprog
		\state{s'}{\conf{\cmdskip;\EBNFthread^*}{\emp}}\\
		\stepprog
		&\state{s'}{\conf{\EBNFthread^*}{\emp}}
	\end{align*}
	By $\EBNFthread\in\EBNFprogramQ$ this yields $\init{\EBNFprogramQ^*}\stepprogany\state{s}{\cfinit{\EBNFprogramQ^*}}\stepprogany\state{s'}{\cfinit{\EBNFprogramQ^*}}$ and thus concludes the claim.
	\qed
\end{proof}

%%%%%%%%%%%%%%%%%%%%%%%%%%%%%%%%%%%%%%%%%%%%%%%%%%%%%%%%%%%%%%%%%%%%%%%%%%%%%%
%%%%%%%%%%%%%%%%%%%%%%%%%%%%%%%%%%%%%%%%%%%%%%%%%%%%%%%%%%%%%%%%%%%%%%%%%%%%%%
%%%%%%%%%%%%%%%%%%%%%%%%%%%%%%%%%%%%%%%%%%%%%%%%%%%%%%%%%%%%%%%%%%%%%%%%%%%%%%

\subsection{Proof of \Cref{thm:fixedpoint:LFP-overapproximates-Reach-P}}

Let $\Program$ be some program and $\Summary$ its summary.
By definition we have $\effects{\Program}\subseteq\effects{\Summary^*}$.
This immediately gives $\Reach{\Program}\subseteq\Reach{\Summary^*}$.
So it remains to show $\Reach{\Summary^*}\subseteq\ReachFP$.
We proceed by induction over the structure of $\Summary^*$ executions.
Fix some arbitrary $\Thread\in\Program$.

\begin{description}[labelwidth=6mm,leftmargin=8mm,itemindent=0mm]
	\item[IB:]
		The empty execution reaches only $\state{\sinit}{\cfinit{\Summary^*}}$.
		By the definition of the fixed point we have $\state{\sinit}{\conf{\Thread}{\emp}}\in X_k$.
		This gives the claim.
		\\[-2mm]

	\item[IH:]
		For every execution $\init{\Summary^*}\stepprogany\state{s}{\cf}$ there is another execution of the form $\init{\Summary^*}\stepprogany\state{s}{\cfinit{\Summary^*}}$ and we have $\state{s}{\conf{\Thread}{\emp}}\in X_k$.
		\\[-2mm]

	\item[IS:]
		Consider now $\init{\Summary^*}\stepprogany\state{s}{\cf}\stepprog[i]\state{s'}{\cf'}$ for some $i$.
		By definition we have $\pair{s}{s'}\in\effects{\Summary^*}$.
		So \cref{auxthm:stateless-effects-give-repeated-executions} together with the induction hypothesis gives the desired $\init{\Summary^*}\stepprogany\state{s}{\cfinit{\Summary^*}}\stepprogany\state{s'}{\cfinit{\Summary^*}}$.
		Hence, the semantics provide $\state{s}{\cfinit{\Summary}}\stepprog\state{s'}{\cf''}$ for some $\cf''$.
		Then, $\state{s'}{\conf{\Thread}{\emp}}\in\Env{X_k}$ holds by definition.
		Thus, $\state{s'}{\conf{\Thread}{\emp}}\in X_k$.
		This concludes the claim.
\end{description}
Consider now some $s\in\Reach{\Summary^*}$.
That is, an execution of the form $\init{\Summary^*}\stepprogany\state{s}{\cf}$ exists.
From the above definition we get $\state{s}{\conf{\Thread}{\emp}}\in X_k$.
Hence, $s\in\ReachFP$.
\qed

%%%%%%%%%%%%%%%%%%%%%%%%%%%%%%%%%%%%%%%%%%%%%%%%%%%%%%%%%%%%%%%%%%%%%%%%%%%%%%
%%%%%%%%%%%%%%%%%%%%%%%%%%%%%%%%%%%%%%%%%%%%%%%%%%%%%%%%%%%%%%%%%%%%%%%%%%%%%%
%%%%%%%%%%%%%%%%%%%%%%%%%%%%%%%%%%%%%%%%%%%%%%%%%%%%%%%%%%%%%%%%%%%%%%%%%%%%%%

\subsection{Proof of \Cref{thm:fixedpoint:sufficient-properties-for-effect-inclusion}}

We have $\stateless{\Summary}$ and $\ReachEff[]{\EBNFthread\inpar\EBNFprogramQ^*}\subseteq\ReachEff[]{\EBNFprogramQ^*}$ for all $\EBNFthread\in\EBNFprogramQ$.
We show that this property implies $\ReachEff[]{\EBNFprogram}\subseteq\ReachEff[]{\EBNFprogram\inpar\EBNFprogramQ^*}\subseteq\ReachEff[]{\EBNFprogramQ^*}$.
The first inclusion holds by definition: $\Program\inpar\Summary^*$ can reach all effects of $\Program$ if the $\Summary^*$ threads stutter.
So consider the second inclusion.
Without loss of generality, let
\begin{align*}
	\cfinit{\EBNFprogram\inpar\EBNFprogramQ^*}&=\cfinit{\EBNFprogram}\uplus\cfinit{\EBNFprogramQ^*}
	\\\text{and}\quad
	\cfinit{\EBNFthread\inpar\EBNFprogramQ^*}&=\set{0\mapsto\conf{\EBNFthread}{\emp}}\uplus\cfinit{\EBNFprogramQ^*}
\end{align*}
in order to avoid the hassle of remapping thread identifiers among executions of different programs.
We now show that for every execution $\init{\EBNFprogram\inpar\EBNFprogramQ^*}\stepprogany\state{s}{\cf}$, every $k\in\dom{\cf}$ and every $\EBNFthread\in\Thrd$ with $\cfinit{\EBNFprogram\inpar\EBNFprogramQ^*}(k)=\conf{\EBNFthread}{\emp}$, there is another execution of the form $\init{\EBNFthread\inpar\EBNFprogramQ^*}\stepprogany\state{s}{\cfinit{\EBNFthread\inpar\EBNFprogramQ^*}[0\to\cf(k)]}$.
In words: in every $\EBNFprogram\inpar\EBNFprogramQ^*$ execution we can replace all $\EBNFprogram$ threads with the present $\EBNFprogramQ^*$ threads.
To do so, statelessness is crucial in order to leverage the $\Summary$ effects for every $\Program$-step that we replace.
We proceed by induction over the structure of the $\EBNFprogram\inpar\EBNFprogramQ^*$ execution.

\begin{description}[labelwidth=6mm,leftmargin=8mm,itemindent=0mm]
	\item[IB:]
		The empty execution reaches only $\sinit$.
		This is true for every program.
		Moreover, the initial configuration is of the desired form.
		\\[-2mm]

	\item[IH:]
		For every $\init{\EBNFprogram\inpar\EBNFprogramQ^*}\stepprogany\state{s}{\cf}$ and $k,\EBNFthread$ with $\cfinit{\EBNFprogram\inpar\EBNFprogramQ^*}(k)=\conf{\EBNFthread}{\emp}$ there is $\init{\EBNFthread\inpar\EBNFprogramQ^*}\stepprogany\state{s}{\cfinit{\EBNFthread\inpar\EBNFprogramQ^*}[0\to\cf(k)]}$.
		\\[-2mm]

	\item[IS:]
		Consider now $\init{\EBNFprogram\inpar\EBNFprogramQ^*}\stepprogany\state{s}{\cf}\stepprog[i]\state{s'}{\cf'}$ for some $i$.
		Let $k,\EBNFthread_k$ be arbitrary with $\cfinit{\EBNFprogram\inpar\EBNFprogramQ^*}(k)=\conf{\EBNFthread_k}{\emp}$.
		We have $\state{s}{\cf(i)}\stepprog\state{s'}{\cf'(i)}$ by the semantics.
		Together with the induction hypothesis for $i$ and some $\EBNFthread_i$ with $\cfinit{\EBNFprogram\inpar\EBNFprogramQ^*}(i)=\conf{\EBNFthread_i}{\emp}$ we have:
		\begin{align*}
			\init{\EBNFthread_i\inpar\EBNFprogramQ^*}
			\stepprogany
			&\state{s}{\cfinit{\EBNFthread_i\inpar\EBNFprogramQ^*}[0\to\cf(i)]}
			\\
			\stepprog[0]
			&\state{s'}{\cfinit{\EBNFthread_i\inpar\EBNFprogramQ^*}[0\to\cf'(i)]}.
		\end{align*}
		For the case $k=i$ this concludes the claim.
		So consider $k\neq i$ now.
		By definition the above $\EBNFthread_i\inpar\EBNFprogramQ^*$ execution gives $\pair{s}{s'}\in\ReachEff[]{\EBNFthread_i\inpar\EBNFprogramQ^*}$.
		If we have $\EBNFthread_i\in\EBNFprogram$, then the premise gives $\pair{s}{s'}\in\ReachEff[]{\EBNFprogramQ^*}$.
		Otherwise, we have $\EBNFthread_i\in\EBNFprogramQ$ and statelessness of $\Summary$ together with \cref{auxthm:stateless-does-not-care-for-duplicated-threads} yields $\pair{s}{s'}\in\ReachEff[]{\EBNFprogramQ^*}$, too.
		Hence, $\stateless{\Summary}$ with \cref{auxthm:stateless-effects-give-repeated-executions} yields: $\state{s}{\cfinit{\EBNFprogramQ^*}}\stepprogany\state{s'}{\cfinit{\EBNFprogramQ^*}}$.
		Together with the induction hypothesis for $k,\EBNFthread_k$ we have:
		\begin{align*}
			\init{\EBNFthread_k\inpar\EBNFprogramQ^*}
			\stepprogany
			&\state{s}{\cfinit{\EBNFthread_k\inpar\EBNFprogramQ^*}[0\to\cf(k)]}
			\\
			\stepprogany
			&\state{s'}{\cfinit{\EBNFthread_k\inpar\EBNFprogramQ^*}[0\to\cf(k)]}.
		\end{align*}
		This concludes the claim because we have $\cf(k)=\cf'(k)$ due to $k\neq i$ together with the semantics.
		\qed
\end{description}

%%%%%%%%%%%%%%%%%%%%%%%%%%%%%%%%%%%%%%%%%%%%%%%%%%%%%%%%%%%%%%%%%%%%%%%%%%%%%%
%%%%%%%%%%%%%%%%%%%%%%%%%%%%%%%%%%%%%%%%%%%%%%%%%%%%%%%%%%%%%%%%%%%%%%%%%%%%%%
%%%%%%%%%%%%%%%%%%%%%%%%%%%%%%%%%%%%%%%%%%%%%%%%%%%%%%%%%%%%%%%%%%%%%%%%%%%%%%

\subsection{Proof of \Cref{thm:fixedpoint:Q-is-summary-of-P}}

Let $X_k$ be the fixed point from \cref{sec:effect-summaries} and let it satisfy the checks \eqref{fp:check:mimic-effects} and \eqref{fp:check:stateless}.
We now show that this implies $\forall\,\Thread\in\Program.~\effects{\Thread\inpar\Summary^*}\subseteq\effects{\Summary^*}$ and $\stateless[]{\Summary}$.
Then, \cref{thm:fixedpoint:sufficient-properties-for-effect-inclusion} yields $\effects{\Program}\subseteq\effects{\Summary^*}$ and we immediately get that $\Summary$ is a summary of $\Program$.

We now proceed by induction over $\Thread\inpar\Summary^*$ executions for some arbitrary thread $\Thread\in\Program$.
Without loss of generality, let
\begin{gather*}
	\cfinit{\Thread\inpar\Summary^*}=\set{0\mapsto\conf{\Thread}{\emp}}\uplus\cfinit{\Summary^*}
\end{gather*}
to avoid remapping thread identifiers of different programs.

\begin{description}[labelwidth=6mm,leftmargin=8mm,itemindent=0mm]
	\item[IB:]
		The empty execution reaches only $\state{\sinit}{\cfinit{\Thread\inpar\Summary^*}}$.
		By definition we have $\state{\sinit}{\cfinit{\Thread\inpar\Summary^*}(0)}=\state{\sinit}{\conf{\Thread}{\emp}}\in X_k$.
		Moreover, $\cfinit{\Summary^*}$ is of the appropriate form.
		\\[-2mm]

	\item[IH:]
		For any $\init{\Thread\inpar\Summary^*}\stepprogany\state{s}{\cf}$ we have $\state{s}{\cf(0)}\in X_k$, $\init{\Summary^*}\stepprogany\state{s}{\cfinit{\Summary^*}}$ and $\cf(i)\in\set{\conf{\Thread^*}{\emp},\conf{\cmdskip}{\emp},\conf{\Thread;\Thread^*}{\emp},\conf{\cmdskip;\Thread^*}{\emp}}$ for every $i\in\dom{\cf}$ with $\cfinit{\Summary^*}(i)=\conf{\Thread^*}{\emp}$.
		\\[-2mm]

	\item[IS:]
		\newcommand{\TT}{{\overline{\Thread}}}
		Consider now an execution of the form $\init{\Thread\inpar\Summary^*}\stepprogany\state{s}{\cf}\stepprog[i]\state{s'}{\cf'}$.
		By definition $i\in\dom{cf}=\dom{\cf'}$.
		First, consider the case $i=0$, that is, $\Thread$ takes a step.
		This immediately gives $\state{s}{\cf'(0)}\in\Post{X_k}\subseteq X_k$ by induction.
		Since $0\notin\dom{\cfinit{\Summary^*}}$ nothing needs to be shown for the third proof obligation.
		From \eqref{fp:check:mimic-effects} we get $\state{s}{\cfinit{\TT}}\stepprog\state{s'}{\cf''}$ for some $\TT\in\Summary$.
		Since $s\in\ReachFP$ follows from the induction hypothesis we have $\cf''=\conf{\cmdskip}{\emp}$ due to \eqref{fp:check:stateless}.
		So the following is valid for some $j$:
		\begin{align*}
			\init{\Summary^*}
			\stepprogany&
			\state{s}{\cfinit{\Summary^*}}
			=
			\state{s}{\cfinit{\Summary^*}[j\to\conf{\TT^*}{\emp}]}\\
			\stepprog&
			\state{s}{\cfinit{\Summary^*}[j\to\conf{\TT;\TT^*}{\emp}]}\\
			\stepprog&
			\state{s}{\cfinit{\Summary^*}[j\to\conf{\cmdskip;\TT^*}{\emp}]}
			=
			\state{s}{\cfinit{\Summary^*}}
		\end{align*}
		This concludes the claim for $i=0$.
		Consider now $i\neq 0$.
		By the semantics we have $\cf(j)=\cf'(j)$ for all $j\neq i$.
		So by induction it suffices for the third proof obligation to show that $\cf'(i)$ is of the appropriate form.
		We do a case distinction on the form of $\cf(i)$ according to the induction hypothesis.
		\\[-2mm]

		\textit{Case $\cf(i)=\conf{\Thread^*}{\emp}.$}
		Due to the semantics of loops we have $s=s'$ and $\cf'(i)\in\set{\conf{\Thread;\Thread^*}{\emp},\conf{\cmdskip}{\emp}}$.
		The former gives $\state{s}{\cf'(0)}\in X_k$ and $\init{\Summary^*}\stepprogany\state{s'}{\cfinit{\Summary^*}}$ by induction.
		The latter shows that $\cf'(i)$ and thus $\cf'$ is of the appropriate form.
		\\[-2mm]

		\textit{Case $\cf(i)=\conf{\cmdskip;\Thread^*}{\emp}.$}
		We have $s=s'$ and $\cf'(i)=\conf{\Thread^*}{\emp}$ by the semantics.
		This concludes the case as before.
		\\[-2mm]

		\textit{Case $\cf(i)=\conf{\cmdskip}{\emp}.$}
		This case cannot apply as it does not allow for the considered step.
		\\[-2mm]

		\textit{Case $\cf(i)=\conf{\Thread;\Thread^*}{\emp}.$}
		We have $\state{s}{\conf{\Thread}{\emp}}\stepprog\state{s'}{\cf''}$ by the semantics for some $\cf''$.
		So $\state{s}{\cfinit{\Summary}}\stepprog[i]\state{s'}{\cfinit{\Summary}[i\to\cf'']}$ is valid.
		Hence, we get the desired $\state{s'}{\cf'(0)}\in\Env{X_k}\subseteq X_k$ by induction.
		Moreover, we have $\cf''=\conf{\cmdskip}{\emp}$ due to \eqref{fp:check:stateless} together with $s\in\ReachFP$ which follows from the induction hypothesis.
		So $\cf'(i)=\conf{\cmdskip;\Thread^*}{\emp}$ is of the appropriate form by the semantics.
		Moreover, the following is valid:
		\begin{align*}
			\init{\Summary^*}
			\stepprogany&
			\state{s}{\cfinit{\Summary^*}}
			=
			\state{s}{\cfinit{\Summary^*}[i\to\conf{\Thread^*}{\emp}]}\\
			\stepprog&
			\state{s}{\cfinit{\Summary^*}[i\to\conf{\Thread;\Thread^*}{\emp}]}\\
			\stepprog&
			\state{s}{\cfinit{\Summary^*}[i\to\conf{\cmdskip;\Thread^*}{\emp}]}
			=
			\state{s}{\cfinit{\Summary^*}}
		\end{align*}
		This concludes the claim.
\end{description}
Now, consider some transition $\state{s}{\cfinit{\Thread}}\stepprog\state{s'}{\cf'}$ with $s\in\Reach{\Summary^*}$.
From the above induction we get $s\in\ReachFP$.
So \eqref{fp:check:stateless} yields $\cf=\conf{\cmdskip}{\emp}$.
Thus, $\stateless{\Summary}$ holds.

Last, consider some effect $\pair{s}{s'}\in\effects{\Thread\inpar\Summary^*}$ for some $\Thread\in\Program$.
There is an execution of the form $\init{\Thread\inpar\Summary^*}\stepprogany\state{s}{\cf}\stepprog[i]\state{s'}{\cf'}$.
The arguments from the induction step above give $\pair{s}{s'}\in\effects{\Summary^*}$ immediately.
\qed
